# Supplementary material for: TripleID-Q: RDF Query Processing Framework using GPU
Source: arXiv:1807.01409 source file (2018-07-04)
Supplement: Supplementary file 1 [file appendix2.tex]

\section{GPUSearch}
 
\label{sec:appendix1}
 Algorithm \ref{al:gpusearch} demonstrated the $GPUSearch$ in Algorithm \ref{al:algorithm1}.
 For each thread, the kernel search is executed using  Algorithm \ref{al:gpusearch}.
The TripleIDs are stored as \texttt{dataArray}, of size multiple of three, in GPU global memory. 
The corresponding thread $i$ compares \texttt{dataArray[i],dataArray[i+1],dataArray[i+2] } to \texttt{key.subj,key.pred,key.obj}.
We represent the output values in binary values as in Table \ref{tab:bit}.

\begin{algorithm}[!htb]{\small{\setstretch{0.6}
\caption{ GPU Search for TripleID  } 
\label{al:gpusearch}
\KwIn{$\textit{dataArray}$, ($\textit{key.subj, key.pred, key.obj}$)}
\KwOut{$\textit{positionArray}$}
 
 		\label{stride}\For{$i =threadIdx;$ $i<n;$ $i += blockDim * gridDim$} 
			{
			 \If{ i \% 3 == 0 } 
 				{
					posidx = (int) i/3; \\

          				  \Case{key.subj==data[i] and key.pred=data[i+1] and  key.obj==data[i+2]  }{
           				    positionArray[ posidx ] =7;	
				          }
				          \Case{key.pred==data[i+1] and  key.obj==data[i+2]} {
				              positionArray[ posidx ] =3;
				          }
				          \Case{key.subj==data[i] and  key.obj==data[i+2] } {
				              positionArray[ posidx ] =5;
				          }
				           \Case{key.subj==data[i] and key.pred==data[i+1] } {
				              positionArray[ posidx ] =6;
				          }
				           \Case{key.subj==data[i] } {
				              positionArray[ posidx ] =4;
				          }
				            \Case{key.pred==data[i+1] } {
				              positionArray[ posidx ] =2;
				          }
				           \Case{key.obj==data[i+2] } {
				              positionArray[ posidx ] =2;
				          }
   		   		         \Other{ positionArray[ posidx ] =0;}
    				      }
								       
			}

}}
\end{algorithm}

\begin{table}[!hbt]\small
\bgroup
{
\caption{Answer bits.}
\label{tab:bit} 
\centering
%\addtolength{\tabcolsep}{-2.5pt}  
\begin{tabular}{|c|c|l|}\hline 
 Binary value&  Decimal	&Meaning \\\hline
 000 & 0 & All matches\\
 001 & 1 & object match (??O) \\
  010 & 2 & predicate match (?P?) \\
   100 & 4 & subject match (S??) \\
   011 & 3 & predicate and object match (?PO) \\
  110 & 6 & subject and predicate match (SP?) \\
   101 & 5 & subject and object match (S?O) \\
    111 & 7 & subject, predicate, object match (SPO) \\\hline
 \end{tabular}\par
}
\egroup
\end{table}

%%%%%%%%%%%%%%%%%%%%%%%%%%%%%%%%%%%%%%%%%%%%%%%%%%%%%%%%%%%%%%%%%%%%%%%%%%%%%
%
%Quesries tested
%
%%%%%%%%%%%%%%%%%%%%%%%%%%%%%%%%%%%%%%%%%%%%%%%%%%%%%%%%%%%%%%%%%%%%%%%%%%%%%
\section{Queries tested}

\label{sec:appendix}
This section presents queries tested in Section \ref{sec:exp}.

\begin{lstlisting}[style=mymatstyle, 
language=SPARQL,
showspaces=false,
basicstyle=\ttfamily,
commentstyle=\color{gray},
caption = {PREFIX list of Q1 - Q16 and R2 - R11},
label = listingprefix]
PREFIX rdf:  <http://www.w3.org/1999/02/22-rdf-syntax-ns#> 
PREFIX owl:  <http://www.w3.org/2002/07/owl#> 
PREFIX rdfs: <http://www.w3.org/2000/01/rdf-schema#>
PREFIX xsd:  <http://www.w3.org/2001/XMLSchema#> 
PREFIX lsr:  <http://lsr.bio2rdf.org/lsr#> 
PREFIX foaf: <http://xmlns.com/foaf/0.1/>
PREFIX data: <http://dig.csail.mit.edu/data#>  
\end{lstlisting}

%Table  \ref{tab:misc3}  presents
%the queries tested in Section \ref{sec:exp}.
%\onecolumn
% \small
%\setlength{\tabcolsep}{0pt}  
%\begin{longtable}{|C{1cm} |L{5cm}| } 
%\caption{Tested Queries. }
%\\ \hline
%\begin{lstlisting}[style=mymatstyle, 
%Q1 & 
%\begin{minipage}{2in}
%
%%PREFIX rdf: <http://www.w3.org/1999/02/22-rdf-syntax-ns#> 
%%PREFIX owl: <http://www.w3.org/2002/07/owl#> 
%%PREFIX rdfs: <http://www.w3.org/2000/01/rdf-schema#>
%%PREFIX xsd: <http://www.w3.org/2001/XMLSchema#> 
%%PREFIX lsr: <http://lsr.bio2rdf.org/lsr#> 
%%\begin{verbatim}
  \begin{lstlisting}[style=mymatstyle, 
language=SPARQL,
showspaces=false,
basicstyle=\ttfamily,
commentstyle=\color{gray},
caption = {Tested Queries: Q1},
label = Q1]
SELECT  * WHERE { 
 ?subject owl:sameAs ?object . 
}  
\end{lstlisting}
%\end{verbatim} 
%\end{minipage} 
%\end{longtable}

  \begin{lstlisting}[style=mymatstyle, 
language=SPARQL,
showspaces=false,
basicstyle=\ttfamily,
commentstyle=\color{gray},
caption = {Tested Queries: Q2},
label = Q2]
SELECT  * WHERE { 
{?subject owl:sameAs ?object . } 
UNION  
{?subject2 rdf:type ?object2 . } 
}
\end{lstlisting}

  \begin{lstlisting}[style=mymatstyle, 
language=SPARQL,
showspaces=false,
basicstyle=\ttfamily,
commentstyle=\color{gray},
caption = {Tested Queries: Q3},
label = Q3]
SELECT  * WHERE { 
{?subject owl:sameAs ?object . } 
 UNION  
{?subject2 rdf:type ?object2 . } 
 UNION   
{?subject3 foaf:name ?object3 . } 
}
\end{lstlisting}

  \begin{lstlisting}[style=mymatstyle, 
language=SPARQL,
showspaces=false,
basicstyle=\ttfamily,
commentstyle=\color{gray},
caption = {Tested Queries: Q4},
label = Q4]
SELECT  * WHERE { 
{?subject owl:sameAs ?object . }
 UNION  
{?subject2 rdf:type ?object2 . } 
 UNION   
{?subject3 foaf:name ?object3. } 
 UNION 
{?subject4 rdfs:subClassOf ?object4 . } 
}
\end{lstlisting}

  \begin{lstlisting}[style=mymatstyle, 
language=SPARQL,
showspaces=false,
basicstyle=\ttfamily,
commentstyle=\color{gray},
caption = {Tested Queries: Q5},
label = Q5]
SELECT  * WHERE { 
data:DIG ?pred ?object .
} 
\end{lstlisting}

  \begin{lstlisting}[style=mymatstyle, 
language=SPARQL,
showspaces=false,
basicstyle=\ttfamily,
commentstyle=\color{gray},
caption = {Tested Queries: Q6},
label = Q6]
SELECT  *  WHERE { 
  { data:DIG ?pred ?object . 
  	FILTER ( regex(str(?pred), "member" ) ) . 
  }  
} 
\end{lstlisting}

  \begin{lstlisting}[style=mymatstyle, 
language=SPARQL,
showspaces=false,
basicstyle=\ttfamily,
commentstyle=\color{gray},
caption = {Tested Queries: Q7},
label = Q7]
SELECT  * WHERE { 
 { data:DIG ?pred ?object .
 	FILTER ( regex(str(?pred), "member" ) ) . 
 } 
 	UNION  
 	{ ?subject2 owl:sameAs ?object2 . 
		 FILTER ( regex( str (?object2),"Croatia" ) ) . 
	} 
} 
\end{lstlisting}

 \begin{lstlisting}[style=mymatstyle, 
language=SPARQL,
showspaces=false,
basicstyle=\ttfamily,
commentstyle=\color{gray},
caption = {Tested Queries: Q8},
label = Q8]
SELECT  * WHERE { 
{ data:DIG ?pred ?object .
 FILTER ( regex(str(?pred), "member" ) ) . 
}  
 UNION  
 { ?subject2 owl:sameAs ?object2 . 
 FILTER ( regex( str (?object2),"Croatia" ) ) .  
 } 
 UNION 
 { ?subject3 foaf:primaryTopic ?object3 . 
 FILTER ( regex( str (?subject3),"foaf" ) ) . 
 } 
} 
\end{lstlisting}

 \begin{lstlisting}[style=mymatstyle, 
language=SPARQL,
showspaces=false,
basicstyle=\ttfamily,
commentstyle=\color{gray},
caption = {Tested Queries: Q9 (SS)},
label = Q9]
SELECT  * WHERE {  
 ?subject <http://dbpedia.org/property/occupation> ?object    . 
 ?subject rdf:type foaf:Person. 
} 
\end{lstlisting}

 \begin{lstlisting}[style=mymatstyle, 
language=SPARQL,
showspaces=false,
basicstyle=\ttfamily,
commentstyle=\color{gray},
caption = {Tested Queries: Q10 (SS SS)},
label = Q10]
SELECT  *  WHERE {  
 ?subject <http://dbpedia.org/property/occupation> ?object     . 
 ?subject rdf:type foaf:Person .  
 ?subject foaf:firstname ?fname      .
} 
\end{lstlisting}

 \begin{lstlisting}[style=mymatstyle, 
language=SPARQL,
showspaces=false,
basicstyle=\ttfamily,
commentstyle=\color{gray},
caption = {Tested Queries: Q11 (SS)},
label = Q11]
SELECT  * WHERE {  
 ?subject <http://vocab.org/relationship/spouseOf> ?object . 
 ?subject foaf:knows ?anyone .  
}
\end{lstlisting}

 \begin{lstlisting}[style=mymatstyle, 
language=SPARQL,
showspaces=false,
basicstyle=\ttfamily,
commentstyle=\color{gray},
caption = {Tested Queries: Q12 (OS)},
label = Q12]
SELECT  * WHERE {  
 ?subject owl:sameAs ?object . 
 ?object  owl:sameAs ?object2.  
}
\end{lstlisting}

 \begin{lstlisting}[style=mymatstyle, 
language=SPARQL,
showspaces=false,
basicstyle=\ttfamily,
commentstyle=\color{gray},
caption = {Tested Queries: Q13 (SS)},
label = Q13]
SELECT  * WHERE {  
 ?subject owl:sameAs ?object  . 
 ?subject owl:sameAs ?object2 .  
} 
\end{lstlisting}

 \begin{lstlisting}[style=mymatstyle, 
language=SPARQL,
showspaces=false,
basicstyle=\ttfamily,
commentstyle=\color{gray},
caption = {Tested Queries: Q14 (SS)},
label = Q14]
SELECT  * WHERE {  
 ?subject owl:sameAs ?object  . 
 ?subject owl:sameAs ?object2 .
 ?subject owl:sameAs ?object3 . 
}
\end{lstlisting}

 \begin{lstlisting}[style=mymatstyle, 
language=SPARQL,
showspaces=false,
basicstyle=\ttfamily,
commentstyle=\color{gray},
caption = {Tested Queries: Q15 (SS)},
label = Q15]
SELECT  * WHERE {  
 ?subject owl:sameAs ?object  . 
 ?subject owl:sameAs ?object2 .
   FILTER ( regex( str (?subject),"us" ) ) .  
}
\end{lstlisting}

 \begin{lstlisting}[style=mymatstyle, 
language=SPARQL,
showspaces=false,
basicstyle=\ttfamily,
commentstyle=\color{gray},
caption = {Tested Queries: Q16 (SS SS SS)},
label = Q16]
SELECT  * WHERE {  
 ?subject owl:sameAs ?object  . 
 ?subject owl:sameAs ?object2 . 
 ?subject owl:sameAs ?object3 . 
 ?subject owl:sameAs ?object4 .
}
\end{lstlisting}

%%%%%%%%%%%%%%%%%%%%%%%%%%%%%%%%%%%%

 \begin{lstlisting}[style=mymatstyle, 
language=SPARQL,
showspaces=false,
basicstyle=\ttfamily,
commentstyle=\color{gray},
caption = {Tested  Entailment Queries: Rule 2},
label = R2]
SELECT * WHERE { 
 ?s ?p ?o          . 
 ?p rdfs:domain ?D . 
}
\end{lstlisting}

 \begin{lstlisting}[style=mymatstyle, 
language=SPARQL,
showspaces=false,
basicstyle=\ttfamily,
commentstyle=\color{gray},
caption = {Tested  Entailment Queries: Rule 3},
label = R3]
SELECT * WHERE { 
 ?s ?p ?o         . 
 ?p rdfs:range ?R . 
}
\end{lstlisting}

 \begin{lstlisting}[style=mymatstyle, 
language=SPARQL,
showspaces=false,
basicstyle=\ttfamily,
commentstyle=\color{gray},
caption = {Tested  Entailment Queries: Rule 5},
label = R5]
SELECT *  WHERE { 
 ?s rdfs:subPropertyOf  ?o  . 
 ?o rdfs:subPropertyOf  ?o2 . 
}
\end{lstlisting}

 \begin{lstlisting}[style=mymatstyle, 
language=SPARQL,
showspaces=false,
basicstyle=\ttfamily,
commentstyle=\color{gray},
caption = {Tested  Entailment Queries: Rule 7},
label = R7]
SELECT * WHERE { 
 ?s ?p                 ?o . 
 ?p rdfs:subPropertyOf ?q . 
}
\end{lstlisting}

 \begin{lstlisting}[style=mymatstyle, 
language=SPARQL,
showspaces=false,
basicstyle=\ttfamily,
commentstyle=\color{gray},
caption = {Tested  Entailment Queries: Rule 9},
label = R9]
SELECT  *  WHERE { 
 ?s rdf:type        ?o  . 
 ?o rdfs:subClassOf ?o2 . 
}
\end{lstlisting}

 \begin{lstlisting}[style=mymatstyle, 
language=SPARQL,
showspaces=false,
basicstyle=\ttfamily,
commentstyle=\color{gray},
caption = {Tested  Entailment Queries: Rule 11},
label = R11]
SELECT * WHERE { 
 ?s rdfs:subClassOf ?o  . 
 ?o rdfs:subClassOf ?o2 . 
}
\end{lstlisting}
